# Supplementary material for: Minimal constraints for Maximum Caliber analysis of dissipative steady state systems
Source: arXiv:1904.11426 source file (2019-07-03)
Supplement: Supplementary file 1 [file Supporting_Info.pdf]

# Supporting Material for:

# Minimal constraints for Maximum Caliber analysis of dissipative steady state systems

Luca Agozzino

*Laufer Center for Physical and Quantitative Biology, Stony Brook University and*

*Department of Physics and Astronomy, Stony Brook University*

Ken Dill

*Laufer Center for Physical and Quantitative Biology, Stony Brook University*

*Department of Physics and Astronomy, Stony Brook University and*

*Department of Chemistry, Stony Brook University*

## I. CALCULATING THE PARTITION FUNCTION

The partition function is given by Eq. 30 of the main text:

$$Z = \sum_X e^{\nu w(X) + \lambda q(X) + \mu \overline{v}(X)} \tag{1}$$

In order to calculate the Lagrange Multiplier, we need to calculate the sum.

First, we express the functions of the trajectory at the exponent for the 3-steps trajectory, which are

$$\overline{v}(X) = v_0 + \frac{2}{3}\xi_1 + \frac{1}{3}\xi_2 \tag{2}$$

$$w(X) = m\xi_1 \left(v_0 + \frac{\xi_1}{2}\right) \delta(\xi_1 - \Delta v_1) + m\xi_2 \left(v_0 + \xi_1 + \frac{\xi_2}{2}\right) \delta(\xi_2 - \Delta v_2) \tag{3}$$

$$q(X) = m\xi_1 \left(v_0 + \frac{\xi_1}{2}\right) \delta(\xi_1 - \Delta u_1) + m\xi_2 \left(v_0 + \xi_1 + \frac{\xi_2}{2}\right) \delta(\xi_2 - \Delta u_2) \tag{4}$$

where the Dirac delta functions assign the correct values to the specific process of energy transfer, whether it is heat or work exchange. The different use of $\Delta v_i$ and $\Delta u_i$ is clarified by Fig.1.

The partition function is therefore

$$Z = \int_{-V_{\max}}^{V_{\max}} dv_0 \int d\xi_1 d\xi_2 \times \tag{5}$$

$$\times \left( \int_{\Delta V_W}^{\Delta V_W} d\Delta v_1 \int_{\Delta V_W}^{\Delta V_W} d\Delta v_2 \; e^{\nu w(X) + \lambda q(X) + \mu \overline{v}(X)} \right. \tag{6}$$

$$+ \int_{\Delta V_W}^{\Delta V_W} d\Delta v_1 \int_{\Delta V_Q}^{\Delta V_Q} d\Delta u_2 \; e^{\nu w(X) + \lambda q(X) + \mu \overline{v}(X)} \tag{7}$$

$$+ \int_{\Delta V_Q}^{\Delta V_Q} d\Delta u_1 \int_{\Delta V_W}^{\Delta V_W} d\Delta v_2 \; e^{\nu w(X) + \lambda q(X) + \mu \overline{v}(X)} \tag{8}$$

$$\left. + \int_{\Delta V_Q}^{\Delta V_Q} d\Delta u_1 \int_{\Delta V_Q}^{\Delta V_Q} d\Delta u_2 \; e^{\nu w(X) + \lambda q(X) + \mu \overline{v}(X)} \right) \tag{9}$$

where the integrals over $\xi_i$ are only used to make use of the delta functions. The limits of integration correspond to the maximum velocities which are allowed by the physics of the system (for example, beyond such values the conduit will break down).

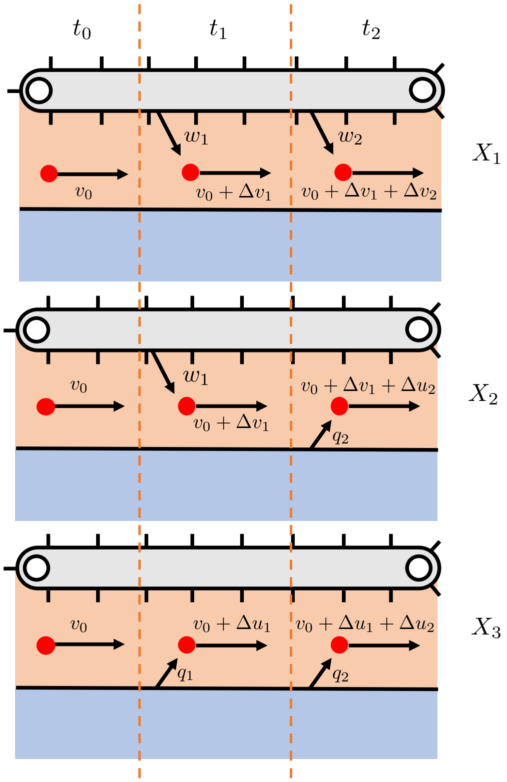


FIG. 1. **Possible trajectories for the 3-step toy model.** $X_1 = \{v_0, \Delta v_1, \Delta v_2\}$ is a trajectory in which all the changes in velocity are due to work exchange (the sign of the change determines the direction of the work flow); $X_2 = \{v_0, \Delta v_1, \Delta u_2\}$ is the trajectory in which first there is exchange of work then heat; $X_3 = \{v_0, \Delta u_1, \Delta u_2\}$ is the trajectory in which there is only heat exchange. Other possible cases include a trajectory without changes and trajectory with more mixed exchanges.

In the MaxCal procedure, the values of the three Lagrange multipliers $\mu, \nu, \lambda$ are unknown until measurements of the average velocity, work and heat are provided, and the following equations are then solved:

$$V = \frac{\partial \ln Z}{\partial \mu} \tag{10}$$

$$E_{\text{in}} = \frac{\partial \ln Z}{\partial \nu} \tag{11}$$

$$-E_{\text{in}} = \frac{\partial \ln Z}{\partial \lambda}. \tag{12}$$

which are the same as Eqs. 20-22 but expressed in terms of the partition function.

From these, and after some approximation we finally obtain

$$\mu \simeq \frac{3\eta}{V} \tag{13}$$

$$\nu \simeq \frac{\epsilon}{2E_{\rm in}} \tag{14}$$

$$\lambda \simeq -\frac{\epsilon}{2E_{\rm in}} \tag{15}$$

where $\eta = V^2/V_{\rm max}^2$ and $\epsilon = \Delta V_Q/\Delta V_W$. $V_{\rm max}$ is the maximum velocity that the conduit can withstand, $\Delta V_Q$ is the maximum change in velocity due to heat exchange and $\Delta V_W$ the one due to heat exchange.
